# Supplementary material for: Partially-averaged Navier-Stokes (PANS) Method for Turbulence Simulations: Near-wall Modeling and Smooth-surface Separation Computations
Source: arXiv:1712.03796 source file (2017-12-11)
Supplement: Supplementary file 1 [file appendices.tex]

%%%%%%%%%%%%%%%%%%%%%%%%%%%%%%%%%%%%%%%%%%%%%%%%%%%
%
%  New template code for TAMU Theses and Dissertations starting Fall 2012.  
%  For more info about this template or the 
%  TAMU LaTeX User's Group, see http://www.howdy.me/.
%
%  Author: Wendy Lynn Turner 
%	 Version 1.0 
%  Last updated 8/5/2012
%
%%%%%%%%%%%%%%%%%%%%%%%%%%%%%%%%%%%%%%%%%%%%%%%%%%%

\begin{appendices}
\titleformat{\chapter}{\centering\normalsize}{APPENDIX \thechapter}{0em}{\vskip .5\baselineskip\centering}

%%%%%%%%%%%%%%%%%%%%%%%%%%%%%%%%%%%%%%%%%%%%%%%%%%%
%
%  New template code for TAMU Theses and Dissertations starting Fall 2012.  
%  For more info about this template or the 
%  TAMU LaTeX User's Group, see http://www.howdy.me/.
%
%  Author: Wendy Lynn Turner 
%	 Version 1.0 
%  Last updated 8/5/2012
%
%%%%%%%%%%%%%%%%%%%%%%%%%%%%%%%%%%%%%%%%%%%%%%%%%%%

%%%%%%%%%%%%%%%%%%%%%%%%%%%%%%%%%%%%%%%%%%%%%%%%%%%%%%%%%%%%%%%%%%%%%%
%%                           APPENDIX A 
%%%%%%%%%%%%%%%%%%%%%%%%%%%%%%%%%%%%%%%%%%%%%%%%%%%%%%%%%%%%%%%%%%%%%

\phantomsection

\chapter{\uppercase{First Appendix}}

Text for the Appendix follows.

\begin{figure}[H]
\centering
\includegraphics[scale=.50]{figures/Penguins.jpg}
\caption{TAMU figure}
\label{fig:tamu-fig5}
\end{figure}

%%%%%%%%%%%%%%%%%%%%%%%%%%%%%%%%%%%%%%%%%%%%%%%%%%%
%
%  New template code for TAMU Theses and Dissertations starting Fall 2012.  
%  For more info about this template or the 
%  TAMU LaTeX User's Group, see http://www.howdy.me/.
%
%  Author: Wendy Lynn Turner 
%	 Version 1.0 
%  Last updated 8/5/2012
%
%%%%%%%%%%%%%%%%%%%%%%%%%%%%%%%%%%%%%%%%%%%%%%%%%%%

%%%%%%%%%%%%%%%%%%%%%%%%%%%%%%%%%%%%%%%%%%%%%%%%%%%%%%%%%%%%%%%%%%%%%%
%%                           APPENDIX B
%%%%%%%%%%%%%%%%%%%%%%%%%%%%%%%%%%%%%%%%%%%%%%%%%%%%%%%%%%%%%%%%%%%%%

\chapter{\uppercase {Second Appendix with a longer title - much longer in fact}}

Text for the Appendix follows.

\begin{figure}[H]
\centering
\includegraphics[scale=.50]{figures/Penguins.jpg}
\caption{TAMU figure}
\label{fig:tamu-fig6}
\end{figure}

\section{Appendix Section}

\pagebreak{}

\end{appendices}
